# Supplementary material for: Adaptation to criticality through organizational invariance in embodied agents
Source: arXiv:1712.05284 ancillary file (2018-06-01)
Supplement: Supplementary file 1 [file Supplementary_Information.pdf]

# Supplementary Information

## Adaptation to criticality through organizational invariance in embodied agents

Miguel Aguilera  
Manuel G. Bedia

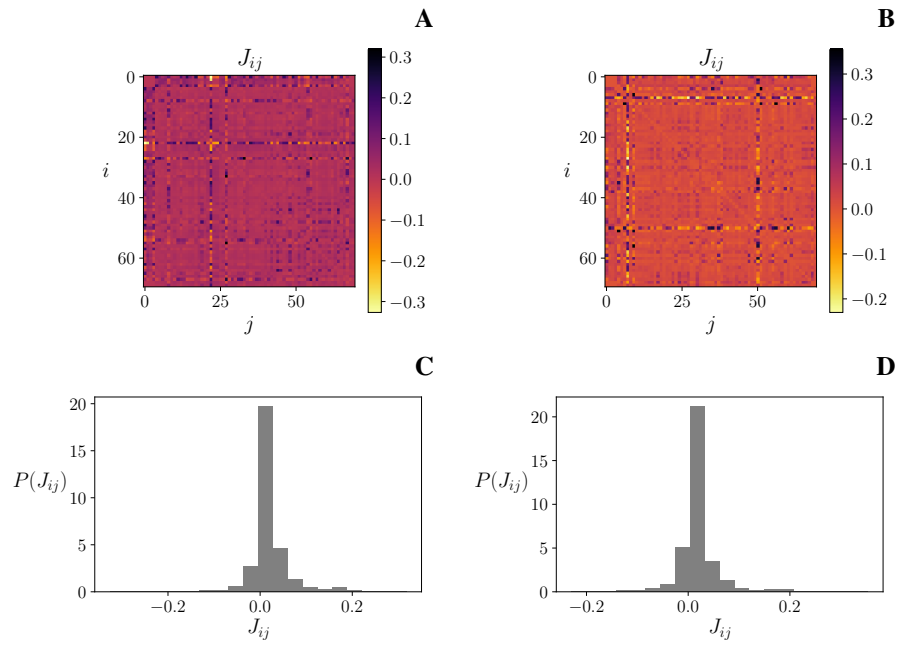

**Figure S1.** Example of the matrix of coupling values  $J_{ij}$  for an agent with  $N_h = 64$  hidden units for the Mountain Car (A) and Acrobot (B) embodiments. (C-D) Histogram of the probability distribution of the corresponding coupling matrix.

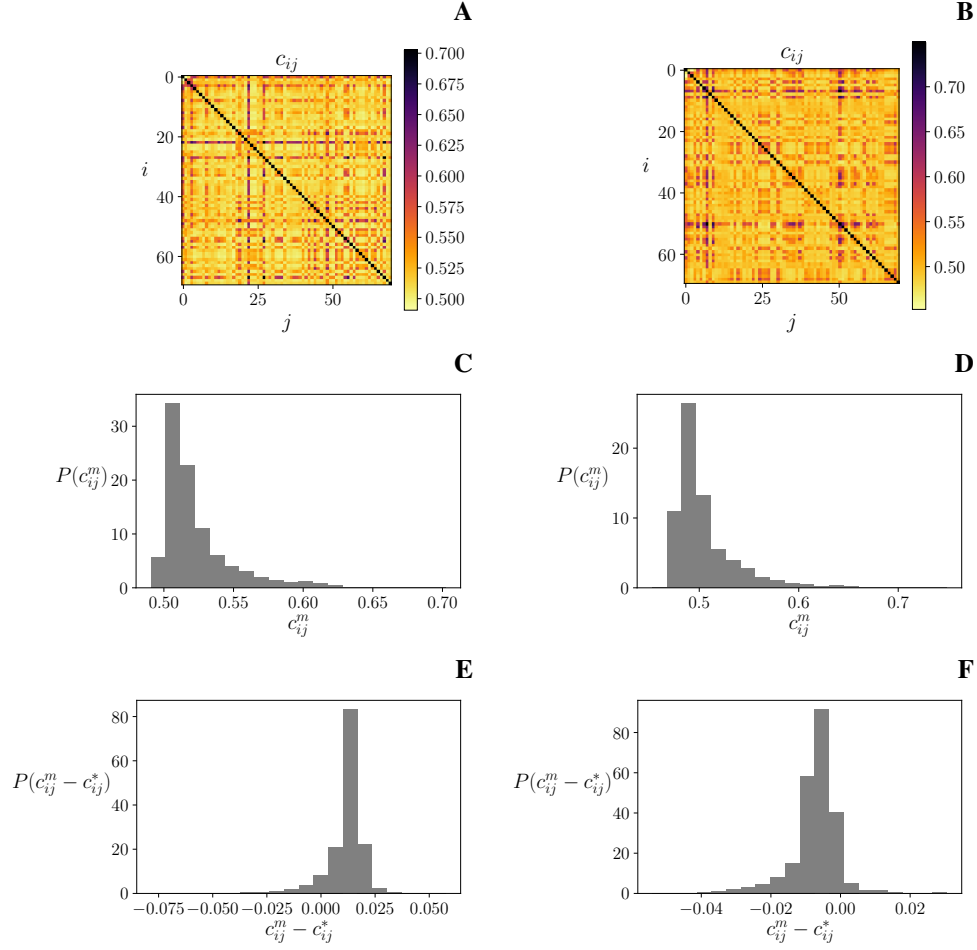

**Figure S2.** Example of the matrix of correlation values  $c_{ij}^m$  for an agent with  $N_h = 64$  hidden units for the Mountain Car (A) and Acrobot (B) embodiments during a simulation of  $10^6$  simulation steps, resetting the agent's position and state every  $5 \cdot 10^4$  simulation steps. (C-D) Histogram of the probability distribution of the corresponding correlation matrix. (C-D) Histogram of the probability distribution of the error between the correlations computed during simulation  $c_{ij}^m$  and reference correlations assigned during training  $c_{ij}^*$ .
